# Supplementary material for: First measurement of $\Xi_{\rm c}^0$ production in pp collisions at $\mathbf{\sqrt{s}}$ = 7 TeV
Source: arXiv:1712.04242 source file (2018-07-12)
Supplement: Supplementary file 1 [file appendix.tex]

\section{Appendix 1}
\label{app:Appendix 1}
